# Supplementary material for: Negative-Weight Single-Source Shortest Paths in Near-linear Time
Source: arXiv:2203.03456 source file (2025-05-20)
Supplement: Supplementary file 1 [file appendix-few_neg_edges.tex]

\section{Proof of Lemma~\ref{thm:prelim:SPWithFewNegEdges}}
Recall that Dijkstra's algorithm executes an initialization step where all distance estimates are set to $\infty$ except the source whose estimate is set to $0$. Our proof will rely on a slight variant of Dijkstra whose initial priority queue contains all vertices with arbitary (possibly negative) initial distance estimates $\disthat(s,u)$ as keys for each $u\in V$. The algorithm updates these distance estimates as edges are relaxed. Note that this variant does not necessarily extract $s$ as the first vertex from the priority queue.

Let $G_+$ denote the graph $G$ with $\eneg(G)$ removed. $\SPWithFewNegEdges(G,s,k)$ initializes $\disthat(s,u)\gets\infty$ for each $u\in V\setminus\{s\}$ and $\disthat(s,s)\gets 0$ (this corresponds to the standard initialization step of Dijkstra). It then executes $k+1$ iterations where each iteration consists of the following two steps: first, run the variant of Dijkstra's algorithm above in $G_+$ (initialized with the current estimates $\disthat(s,u)$); then relax all edges in $\eneg(G)$, updating estimates $\disthat(s,u)$ further.

Clearly, $\SPWithFewNegEdges(G,s,k)$ has the desired running time. Since edge relaxations are the only operations that update distance estimates and since for each $v\in V$, $\dist(s,v)\leq 0$, we have $0\geq\disthat(s,v)\geq\dist(s,v)$.

It remains to show that for each $v$ that is $(s,k)$-negative in $G$, we have $\disthat(s,v) = \dist(s,v)$. The shortest path $P = P(v;G,s)$ contains at most $k$ negative edges of $\eneg(G)$. Partition this path into maximal subpaths each of which is either contained in $G_+$ or consists of a single negative edge; let $P_1,e_1,P_2,e_2,\ldots,e_{r-1},P_r$ be these subpaths in order along $P$, where each $P_i$ is contained in $G_+$ and each $e_i\in\eneg(G)$ (possibly with some $P_i$-paths consisting of a single vertex). We have $r\leq k+1$.

Denote by $s_i$ and $t_i$ the first and last vertex of $P_i$, respectively, for each $i$. We will show by induction on $i\in\{1,2,\ldots,r\}$ that after the $i$th iteration of $\SPWithFewNegEdges(G,s,k)$, $\disthat(s,u) = \dist(s,u)$ for each vertex $u$ of $P_i$ as well as for the vertex $s_{i+1}$ if it exists (i.e., if $i < r$).

We first consider the base case $i = 1$. After Dijkstra has been executed, $\disthat(s,u) = \dist(s,u)$ for each vertex $u$ of $P_1$; this is immediate from the correctness of Dijkstra. Since $e_1$ is subsequently relaxed, we have $\disthat(s,s_2) = \dist(s,s_2)$ at the end of the first iteration. This shows the base case.

Now assume $i > 1$ and that the claim holds for smaller values. In particular, $\disthat(s,s_i) = \dist(s,s_i)$. Note that Dijkstra's algorithm is executed on $G_+$. A simple modification of the correctness proof of Dijkstra then shows that our variant of Dijkstra relaxes the edges of $P_i$ in order. Hence, afterwards, $\disthat(s,u) = \dist(s,u)$ for each vertex $u$ of $P_i$. If $i < r$, the subsequent relaxation of $e_i$ ensures that $\disthat(s,s_{i+1}) = \dist(s,s_{i+1})$. This completes the inductive step.

It follows that at termination, $\disthat(s,v) = \dist(s,v)$ for the last vertex $v$ of $P$, as desired.
