# Supplementary material for: Negative-Weight Single-Source Shortest Paths in Near-linear Time
Source: arXiv:2203.03456 source file (2025-05-20)
Supplement: Supplementary file 2 [file appendix-spaverage.tex]

\section{Proof of Lemma \ref{lem:spaverage} ($\SPaverage$)}
\label{sec:app:spaverage}
\spaverageLemma*
We will implement $\SPaverage(G)$ to compute distance estimates $d(v)$ so that at termination, $d(v) = \dist_{G_s}(s,v)$ for each $v\in V$; then, by Lemma \ref{lem:price-equivalent}, we can output $\phi(v) = \dist_{G_s}(s,v)$. We also need to ensure that the algorithm does not terminate if there is a negative cycle. To simplify notation, throughout this entire section we let $G$ refer to $G_s$, let $s$ refer to the dummy source, and let $\dist$ refer to $\dist_{G_s}$.

\subsection{The algorithm}
Full pseudocode is given in Algorithm \ref{alg:spaverage}. The priority queue $Q$ is implemented as a binary heap, supporting each queue operation in $O(\log n)$ time.

\begin{algorithm2e}[h] 
\label{alg:spaverage}
	\caption{Algorithm for $\SPaverage(G)$}
Set $d(s) \gets 0$ and $d(v) \gets \infty$ for $v \neq s$

Initialize priority queue $Q$ and add $s$ to $Q$.

Initially, every vertex is unmarked %\tcp*[f]{Vertex $v$ will be marked if $d(v)$ changes during a phase.}

\BlankLine

\tcp*[h]{\textcolor{blue}{Dijkstra Phase}}

\While(\label{line:dijkstra-phase}){Q is non-empty}{

Let $v$ be the vertex in $Q$ with minimum $d(v)$

Extract $v$ from $Q$ and mark $v$

\ForEach{edge $(v,x) \in E \setminus \eneg(G)$}{

\If{$d(v) + w(v,x) < d(x)$}{

Mark $x$ and add $x$ to $Q$ \tcp*[f]{$x$ may already be marked or in $Q$.}

$d(x) \gets d(v) + w(v,x)$

} %EndIf
} %end ForEach
} %end While

\tcp*[h]{\textcolor{blue}{Bellman-Ford Phase}}

\ForEach{marked vertex $v$}{
\ForEach{edge $(v,x) \in E^{neg}(G)$}{
\If{$d(v) + w(v,x) < d(x)$}{

$d(x) \gets d(v) + w(v,x)$

Add $x$ to $Q$

} %end If
} %end ForEach
Unmark $v$
} %End ForEach

If $Q$ is empty: \Return $d(v)$ for each $v\in V$ \tcp*[f]{labels do not change so we have correct distances.}

Go to Line \ref{line:dijkstra-phase} \tcp*[f]{$Q$ is non-empty.}

\end{algorithm2e}
In the following, we say that an edge $(v,x)$ of $G$ is \emph{active} if $d(v) + w(v,x) < d(x)$ and \emph{inactive} otherwise. Note that $(v,x)$ is inactive after being relaxed, i.e., after assigning $\min\{d(x), d(v) + w(v,x)\}$ to $d(x)$, and can only become active again if $d(v)$ is reduced.

We define an iteration of the algorithm as a single execution of a Dijkstra Phase followed by a Bellman-Ford Phase. The initial iteration is referred to as iteration $0$, the next iteration is iteration $1$, and so on.

\subsection{Correctness}
For the correctness and running time analysis, the following lemma will be useful.
\begin{lemma}\label{lemma:InactiveEdges}
Just after any execution of the Dijkstra Phase, all edges of $E\setminus\eneg(G)$ are inactive. Just after any execution of the Bellman-Ford Phase, all edges of $\eneg(G)$ are inactive.
\end{lemma}
\begin{proof}
The proof is by induction on the iteration $i\geq 0$. Assume first that $i = 0$. Then the first part of the lemma follows from the analysis of Dijkstra's algorithm. Since $s$ is a dummy source, all vertices will have been marked just prior to the Bellman-Ford Phase so the second part of the lemma follows as well. 

Now, assume that $i > 0$ and that the lemma is true for iteration $i-1$. Observe that the Bellman-Ford Phase in iteration $i-1$ added to $Q$ every vertex whose distance estimate was decreased in that phase. By the induction hypothesis, only edges outgoing from these vertices can be active at the beginning of iteration $i$. The analysis of Dijkstra's algorithm ensures that all such edges belonging to $E\setminus \eneg(G)$ are inactive at the end of the Dijkstra Phase of iteration $i$, showing the induction step for the first part of the lemma. The Dijkstra Phase in iteration $i$ marks every vertex whose distance estimate was reduced in that phase or whose distance estimate was reduced in the Bellman-Ford Phase of iteration $i-1$ (since vertices extracted from $Q$ are marked). These marked vertices are exactly those for which outgoing edges of $\eneg(G)$ can be active just after the Dijkstra Phase in iteration $i$. Since the Bellman-Ford Phase in iteration $i$ relaxes all edges of $\eneg(G)$ outgoing from marked vertices, the induction step also holds for the second part of the lemma.
\end{proof}
\begin{corollary}\label{cor:InactiveAtTermination}
If the algorithm terminates, all edges are inactive.
\end{corollary}
\begin{proof}
Assume there is a final iteration $i$. By Lemma~\ref{lemma:InactiveEdges}, all edges of $E\setminus\eneg(G)$ are inactive after the Dijkstra Phase and all edges of $\eneg(G)$ are inactive after the Bellman-Ford Phase. Since the latter phase did not add any vertices to $Q$ (otherwise, the algorithm would not terminate in iteration $i$), the Bellman-Ford Phase could not have made any edges of $E\setminus\eneg(G)$ active.
\end{proof}
The following lemma shows correctness when there are negative cycles.
\begin{lemma}\label{lemma:NoTerminationWithNegCycle}
If $G$ has a negative cycle, the algorithm never terminates.
\end{lemma}
\begin{proof}
The proof is by contraposition. Suppose the algorithm terminates and let $C$ be a cycle of $G$. By Corollary~\ref{cor:InactiveAtTermination}, all edges are inactive at this point. Thus,
\[
\sum_{(u,v)\in E(C)} w(u,v) = \sum_{(u,v)\in E(C)}(\dist(s,u) + w(u,v) - \dist(s,v))\geq 0,
\]
so $C$ is not a negative cycle.
\end{proof}
It remains to show correctness in the absence of negative cycles. By Corollary~\ref{cor:InactiveAtTermination}, it suffices to show that the algorithm terminates in this case. However, we will show a stronger result that will be needed in the running time analysis. For each $v\in V$ and each integer $i\geq 0$, define $\dist_i(v)$ to be the weight of a shortest path from $s$ to $v$ among all $s$-to-$v$ paths in $G$ containing at most $i$ edges of $\eneg(G)$.
\begin{lemma}\label{lemma:DistAfterDijkstraPhase}
If $G$ has no negative cycles then after the Dijkstra Phase in iteration $i\geq 0$, $d(v)\leq \dist_i(s,v)$ for each $v\in V$.
\end{lemma}
\begin{proof}
The proof is by induction on $i\geq 0$. The base case $i = 0$ follows from the first part of Lemma~\ref{lemma:InactiveEdges} so assume $i > 0$ and that the lemma holds for iteration $i-1$. Let $v\in V$ be given. %We may assume that $d(v) > \dist_i(s,v)$ at the beginning of iteration $i$.

Let $P$ be a shortest path from $s$ to $v$ among all $s$-to-$v$ paths in $G$ containing at most $i$ edges of $\eneg(G)$; $P$ exists since $s$ is a dummy source. We may assume that $P$ has exactly $i$ edges of $\eneg(G)$ since otherwise the induction hypothesis implies $d(v)\leq \dist_{i-1}(s,v) = \dist_i(s,v)$ after the Dijkstra Phase in iteration $i-1$ and hence also after the Dijkstra Phase in iteration $i$.

Partition $P$ into maximal subpaths each of which either contains only edges of $E\setminus\eneg(G)$ or consists of a single edge from $\eneg(G)$. Let $P_0,e_0,P_1,e_1,\ldots,e_{i-1},P_{i}$ be these subpaths where each $P_j$ contains only edges from $E\setminus\eneg(G)$ and each $e_j\in\eneg(G)$ (possibly with some subpaths $P_j$ consisting of a single vertex). Let $s_j$ resp.~$t_j$ be the first resp.~last vertex of subpath $P_j$.

Let $j$ be the first iteration in which $d(t_{i-1}) \leq \dist_{i-1}(s,t_{i-1})$ just after the Dijkstra Phase; by the induction hypothesis, $j\leq i-1$. We show in the following that $t_{i-1}$ is marked just after this Dijkstra Phase.

If the Dijkstra Phase of iteration $j$ reduced $d(t_{i-1})$, it marked $t_{i-1}$ so assume otherwise. Then the minimality of $j$ ensures that the Bellman-Ford Phase of iteration $j-1$ reduced $d(t_{i-1})$; in this case, $t_{i-1}$ must belong to $Q$ at the beginning of iteration $j$ and hence $t_{i-1}$ is marked when it is extracted from $Q$ in the Dijkstra Phase of iteration $j$.

We conclude that $t_{i-1}$ is marked just after the Dijkstra Phase of iteration $j$ so the subsequent Bellman-Ford Phase relaxes $(t_{i-1},s_i)$. This ensures that at the beginning of iteration $j+1$ and hence at the beginning of iteration $i$, $d(s_i)\leq \dist_i(s,s_i)$. By the first part of Lemma~\ref{lemma:InactiveEdges}, $d(v)\leq \dist_i(s,v)$ after the Dijkstra Phase in iteration $i$. This shows the induction step.
\end{proof}
Since Lemma~\ref{lemma:DistAfterDijkstraPhase} in particular implies that the algorithm terminates when there are no negative cycles in $G$, correctness now follows from Corollary~\ref{cor:InactiveAtTermination}:
\begin{corollary}
If $G$ has no negative cycles, the algorithm terminates with $d(v) = \dist(s,v)$ for each $v\in V$.
\end{corollary}

\subsection{Running time}
By Lemma~\ref{lemma:NoTerminationWithNegCycle}, it suffices to analyze the running time for the case where $G$ has no negative cycles. Recall the input assumption that all vertices in $G$ have constant out-degree. Observe that every time a vertex is marked, it is either added to or extracted from $Q$. Furthermore, for every vertex extracted from $Q$ in the Dijkstra Phase and for every marked vertex processed in the outer for-loop of the Bellman-Ford Phase, only a constant number of outgoing edges exist so only $O(\log n)$ time is required to process each such vertex, where the dominant part in the time bound is the update of $Q$. Since the number of extractions from $Q$ cannot exceed the number of insertions, it thus suffices to show that the number of insertions into $Q$ is $O(\sum_{v \in V} \eta_G(v))$.

Each vertex $v$ is added to $Q$ at most twice per iteration, namely at most once in each of the two phases. Hence, if $\dist(s,v) = \dist_i(s,v)$, Lemma~\ref{lemma:DistAfterDijkstraPhase} implies that $v$ is added to $Q$ only $O(i+1)$ times during the course of the algorithm: $d(v) = \dist(s,v)$ after the Dijkstra Phase of the $(i+1)$th iteration, after which $d(v)$ never changes again and is consequently never added to $Q$. Since $\dist_{\eta_G(v)} = \dist(s,v)$, $v$ is added to $Q$ only $O(\eta_G(v)+1)$ times. Over all $v\in V$, this is $O(\sum_{v\in V}(\eta_G(v)+1)) = O(n + \sum_{v\in V}\eta_G(v))$. Multiplying by the $O(\log n)$ time per queue operation gives the time bound.
